# Supplementary material for: Global Optimization, Local Adaptation, and the Role of Growth in Distribution Networks
Source: arXiv:1606.00331 ancillary file (2016-09-22)
Supplement: Supplementary file 1 [file supplemental-material.pdf]

# Supplemental Material for "Global optimization, local adaptation and the role of growth in distribution networks"

Henrik Ronellenfitsch* and Eleni Katifori†
*Department of Physics and Astronomy, University of Pennsylvania, Philadelphia, PA 19104, USA.*
(Dated: August 24, 2016)

## I. TISSUE MATRIX GROWTH

Our model of network adaptation on a growing tissue matrix consists of two layers of dynamics. The first layer consists of modeling the growth of the underlying tissue and the second of the adaptation of the venation. In this section we discuss the first layer of modeling, the tissue matrix. The sole effect of the growing tissue matrix is to introduce time-dependent scaling factors into the dynamical equations. In what follows, we will focus on 2D systems, but the results can be easily generalized to 3D.

Following [1] (and others), we model the cells of the growing leaf lamina as a two-dimensional expanding viscous fluid in mechanical equilibrium. During growth in leaves and other 2D tissues the thickness increases as well, but we take this growth to be negligibly small. Let the position of a small volume element of cells be given by $\mathbf{x}(t)$ and its velocity by $\mathbf{v}(t) = \dot{\mathbf{x}}(t)$. Assuming that the cell number density is constant and all cells are approximately equally sized, the dynamics is governed by the continuity equation

$$\nabla \cdot \mathbf{v} = r, \tag{1}$$

where $r$ is the constant rate of isotropic cell division. In the absence of external forces, the force balance reads

$$\partial_k(\sigma_{ik} - P\delta_{ik}) = 0, \tag{2}$$

where $P$ is the pressure and we assume a viscous stress tensor

$$\sigma_{ik} = \eta\left(\partial_i v_k + \partial_k v_i - \delta_{ik}\partial_s v_s\right) + \zeta\delta_{ik}\partial_s v_s. \tag{3}$$

Here, $\eta$ is the shear viscosity and $\zeta$ is the bulk viscosity. At the boundary of the tissue, we impose the conditions $\sigma_{nn} = P - P_{\text{ext}}$ and $\sigma_{nt} = 0$, where $\sigma_{nn}$ is the normal component of stress, $\sigma_{nt}$ is the tangential component, and $P_{\text{ext}}$ is the external pressure. Further assuming uniform pressure, the continuum tissue dynamics can be solved to yield

$$\mathbf{x}(t) = e^{\frac{r}{2}t}\mathbf{x}_0 = \lambda_t \mathbf{x}_0, \tag{4}$$

where we introduced the scaling factor $\lambda_t = e^{\frac{r}{2}t}$. We note that the distance between two reference points scales as $L(t) = \|\mathbf{x}(t) - \mathbf{y}(t)\| = \lambda_t L(0)$.

## II. ANIMAL VASCULATURE

Animal vasculature is able to adapt to changing conditions both during development and in the adult body [2]. In this section, we show in which ways our model, presented in the main paper, is related to standard models of vascular adaptation.

In blood vessels the volume flow $F_e$ through a vein of length $L_e$ connecting nodes $i$ and $j$ follows approximately Poiseuille's law

$$F_e = c\mu\frac{r_e^4}{L_e}(p_j - p_i) = \frac{K_e}{L_e}(p_j - p_i), \tag{5}$$

* henrikr@sas.upenn.edu
† katifori@sas.upenn.edu

where $c$ is a constant, $\mu$ is the dynamic viscosity of blood, and $p_i$ is hydrostatic pressure at node $i$. Blood vessels are then believed to mainly respond to wall shear stress [3]

$$\tau_e \sim \frac{F_e}{r_e^3}, \tag{6}$$

by adjusting their vessel diameter. One popular model for this behavior is

$$\frac{dr_e}{dt} = c' \left( |\tau_e|^\sigma - \tau_d^\sigma \right) r_e, \tag{7}$$

where $\tau_d$ is some desired value of the wall shear stress and $\sigma$ is a parameter. Using the fact that $r_e \sim K_e^{1/4}$, we rewrite this equation to read

$$\frac{dK_e}{dt} = c'' \left( |F_e|^\sigma K_e^{1-3\sigma/4} - \tau_d^\sigma K_e \right). \tag{8}$$

This is directly related to the model used in [4]. We are interested in the steady state $K_{ij}$'s. Equivalent steady states are obtained from the equation

$$\frac{dK_e}{dt} = c''|F_e|^{4/3} - c''\tau_d^{4/3} K_e. \tag{9}$$

Thus, the steady states of any generalized vascular remodeling equation are equivalent to those obtained from the adaptation equation discussed in the main paper with $\gamma = 2/3$ and any finite value of $\rho$.

The two augmented adaptation rules

$$\frac{dK_e}{dt} = a|F_e|^\sigma K_e^{1-3\sigma/4} - bK_e + c \tag{10}$$

$$\frac{dK_e}{dt} = a|F_e|^{2\gamma} - bK_e + c \tag{11}$$

exhibit qualitatively similar transients when taking into account growth (the transients described in the main paper), and their steady states minimize the energy functional given in the main paper in this case as well. Equations 10 and 11 belong to an extended family of such rules with similar dynamics.

We note that the constant background production term is absent from equation (9). In general, a constant background production term results in non-vanishing steady state conductivities even in the absence of flow, and can be thought to correspond to the presence of an angiogenic growth factor.

## III. PLANT VEIN MORPHOGENESIS

Plant veins are widely believed to develop through a mechanism called auxin canalization. In the simplest, non-polar model from [5], the morphogen auxin flows between cells according to

$$F_e = \frac{K_e}{L_e}(\phi_j - \phi_i), \tag{12}$$

where $K_e$ is a facilitated diffusion constant, $\phi_i$ is auxin concentration at node $i$, $L_e$ is the distance over which auxin diffuses and $F_e$ is auxin flow. The facilitated diffusion constants are thought to represent transporter proteins (in particular, PIN1) which are responsible for carrying auxin. In the simplest case they are thought to follow an adaptation equation of the form

$$\frac{dK_e}{dt} = a|F_e|^\sigma - bK_e + c, \tag{13}$$

which directly corresponds to equation (4) in the main paper. This adaptation creates a steady state pattern of auxin flow. Cells in the leaf primordium are then believed to detect this pattern and accordingly modify into vascular cells where $K_e$ is large.

# IV. ENERGY FUNCTIONAL

## A. Volume constraint

The optimization functional can be written as

$$E = \sum_e L_e \frac{F_e^2}{K_e} + \mu \left( \sum_e L_e K_e^{\frac{1}{\gamma}-1} - C \right), \tag{14}$$

where $\mu$ is a Lagrange multiplier and $C$ is a constant. If we assume Poiseuille-like flow, $K_e \sim r^4$, and the constraint can be seen to be equivalent to fixing the total network volume if $\frac{1}{\gamma} - 1 = 1/2$, i.e., if $\gamma = 2/3$. This is the assumption for animal networks as well as for the final, fully developed plant venation.

## B. Scaling of the energy

The energy functional scales as

$$E = \lambda_t^{2\delta+1-\tau} \left( \sum_e L'_e \frac{(F'_e)^2}{K'_e} + \lambda_t^{\frac{\tau}{\gamma}-2\delta} \mu \left( \sum_e L'_e (K'_e)^{\frac{1}{\gamma}-1} - \lambda_t^{-\frac{\tau}{\gamma}+\tau-1+\sigma} C' \right) \right), \tag{15}$$

with the constraint value scaling as $C = \lambda_t^{\sigma} C$ with $\sigma$ unknown. In order for the energy to be consistent (i.e, it should satisfy a scaling relation $E = \lambda_t^{\nu} E'$, where $E'$ remains finite and retains the constraint term for $t \to \infty$) we need $\tau = 2\gamma\delta$, just as we derived from the adaptation equation directly in the main paper. The constraint value must therefore scale as $C = \lambda_t^{2\delta(1-\gamma)+1} C'$. We find

$$E = \lambda_t^{2\delta(1-\gamma)+1} \left( \sum_e L'_e \frac{(F'_e)^2}{K'_e} + \mu \left( \sum_e L'_e (K'_e)^{\frac{1}{\gamma}-1} - C' \right) \right) = \lambda_t^{2\delta(1-\gamma)+1} E'. \tag{16}$$

# V. NONDIMENSIONALIZATION OF THE MODEL

We nondimensionalize the system of equations (5,7) presented in the main manuscript as follows:

$$K' = \frac{a}{b'} (\hat{S}/\hat{F})^{2\gamma} \tilde{K}, \quad t = \frac{1}{b'} \tilde{t}, \quad \mathbf{F}' = \hat{S} \tilde{\mathbf{F}}$$
$$L' = \hat{L} \tilde{L}, \quad \mathbf{S}' = \hat{S} \tilde{\mathbf{S}}. \tag{17}$$

The definitions of the symbols follow the main manuscript. Quantities with a tilde are dimensionless and quantities with a hat are typical scales. The model equations then reduce to the dimensionless system

$$\tilde{\mathbf{F}} = \tilde{K} \tilde{L}^{-1} \Delta \left( \Delta^T \tilde{K} \tilde{L}^{-1} \Delta \right)^{\dagger} \tilde{\mathbf{S}} \tag{18}$$

$$\frac{d\tilde{K}_e}{d\tilde{t}} = \tilde{F}_e^{2\gamma} - \tilde{K}_e + \kappa \exp(-\tilde{t}/(1+\rho)), \tag{19}$$

with the dimensionless control parameters $\kappa = (c/a)(\hat{F}/\hat{S})^{2\gamma}$, $\rho = b/(r\gamma\delta)$.

# VI. STERIC CONSTRAINTS

Because conductivities and underlying tissue grow at different rates, it is possible that at some time $t_s$ the radii of animal blood vessels become so large that they overlap. At this point, our model ceases to be valid. However, we now show that this case can always be avoided by an appropriate choice of parameters.

We estimate that the steric constraint is violated once the typical vessel radius, marked with a bar, $\bar{R}(t) \approx \lambda_t \hat{L}$, becomes comparable to the typical vessel length scale. Because $\bar{K}(t) = z\bar{R}(t)^4$ and $\bar{K}(t) = \lambda_{t_s}^{2\gamma\delta} \hat{K}$, this condition can be rewritten as

$$\lambda_{t_s}^{2\gamma\delta} \hat{K} \approx z \lambda_{t_s}^4 \hat{L}^4. \tag{20}$$

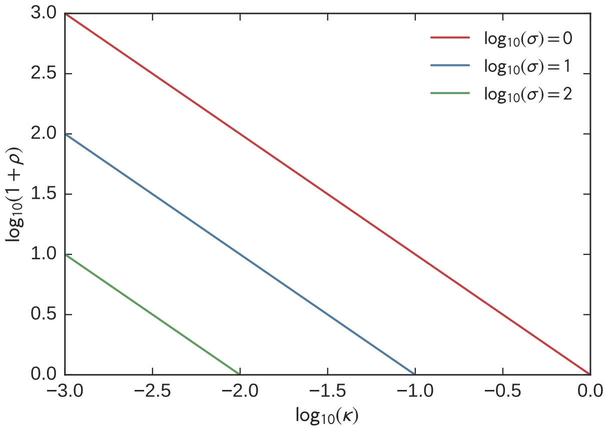


FIG. 1. Estimated steric constraints in parameter space. The allowed region of parameter space for a given value of $\sigma$ is the half-plane above the respective line.

Using (17) and remembering that $K' = \hat{K}\tilde{K}$, this can be expressed in terms of dimensionless control parameters as

$$\lambda_{t_s}^{2\gamma\delta-4} \approx z\hat{L}^4 \frac{b + r\gamma\delta}{a} \left(\frac{\hat{F}}{\hat{S}}\right)^{2\gamma} = \kappa\,(1+\rho)\,\sigma, \tag{21}$$

where $\sigma = \gamma\delta z\hat{L}^4 r/c$. Because $1/2 < \gamma < 1$ and typically $\delta = 2$ for 2d tissues, the LHS is monotonically decreasing and bounded above by 1. Thus, in order for the steric constraint to be irrelevant, the RHS must be greater than 1.

The RHS of (21) can be increased by increasing the value of $\sigma$ independently from the other dimensionless parameters in order to satisfy the constraint. We note that in real plants and animals, the steric constraint may influence the possible values of the dimensionful parameters and the initial conditions and may thus restrict the dynamics.

In log-space the steric constraint can be written as

$$\log_{10}(\kappa) + \log_{10}(1+\rho) + \log_{10}(\sigma) > 0. \tag{22}$$

We plot the associated lines in parameter space in Fig. 1. The allowed region is given by the half planes above the lines. Thus, we see that a value of $\sigma = 1000$, the entire parameter space explored in the main paper is allowed. Because the prefactor $\gamma\delta$ is bounded below by 1, this corresponds to a lower limit to the ratio of length growth per time to background production of vessel radius per time of $\sqrt[4]{1000} \approx 5.6$, which is reasonable, and one may expect this ratio to be much larger in real systems. Further, it is highly interesting to note that for lower values of $\sigma$, the steric constraint forbids high energy regions, i.e., non-optimal networks, in parameter space.

For 3d tissues, $\delta = 3$ such that the LHS of (21) may become increasing and the steric constraint may become relevant.

## VII. SIMULATED ANNEALING

We employ a version of the annealing algorithm from [6]. At each annealing step, the network is first optimized using a steepest descent method. Then, the result is convolved with a Gaussian kernel

$$k(e,f) = \exp\left(-\frac{d(e,f)^2}{2\beta}\right), \tag{23}$$

where $d(e,f)$ is the Euclidean distance between the centers of edges $e$ and $f$, and $\beta$ is a parameter that is successively decreased. The range of $\beta$ varies from the order of the system size to the order of less than one edge length during the algorithm. Finally, we add multiplicative noise as $K_e \to \exp(s\xi)K_e$, where $s$ is a parameter and $\xi$ is taken from the standard normal distribution.

For the results in this paper, we additionally randomize the total number of steps used to decrease $\beta$ between 200 and 800, and repeat the process 1000 times to obtain a highly optimized final network.

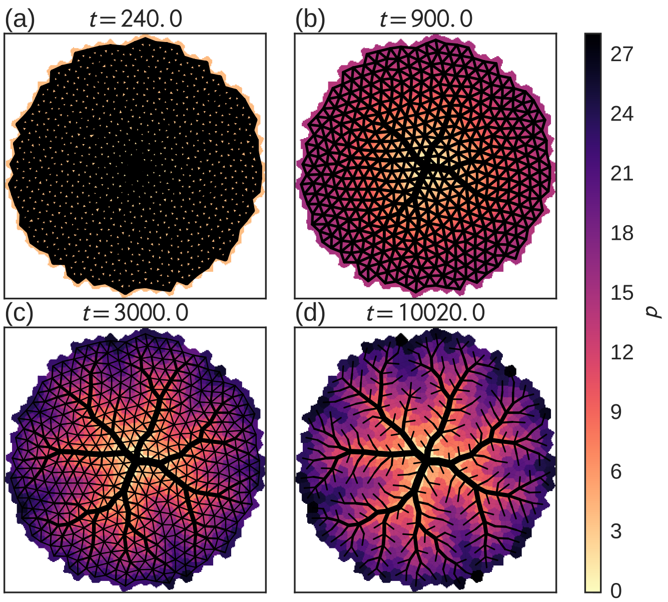


FIG. 2. Adaptation dynamics for a polynomial growth law with $n = 1$.

## VIII. EXPLORATION OF OTHER GROWTH LAWS

In the main paper we used exponential growth, $\lambda_t = e^{rt/2}$, but the model is robust also for other growth laws as long as they are subexponential, i.e., as long as $\dot{\lambda}_t/\lambda$ is either constant or tends to zero. Here, we show the model dynamics with linear and quadratic growth laws. For general polynomial growth laws we can write

$$\lambda_t = 1 + \frac{1}{n}(rt)^n \tag{24}$$

$$\dot{\lambda}_t = r(rt)^{n-1}. \tag{25}$$

We show the typical dynamics under those growth laws in Figs. 2, 3 for $n = 1, 2$, where we use the dimensionless adaptation equation

$$\frac{dK_e}{dt} = F_e^{2\gamma} - \left(1 + \rho\frac{\dot{\lambda}_t}{r\lambda_t}\right) K_e + \kappa\lambda_t^{-2\gamma\delta}, \tag{26}$$

with $\rho = 0.1$, $\kappa = 1$, $r = 0.01$, $\delta = 2$ and $\gamma = 2/3$. We conclude that the qualitative dynamics which optimizes the network is robust under changes of the growth law. However, the absolute time scale over which adaptation occurs differs.

## IX. EXPLORATION OF OTHER LATTICES

In this section, we explore the phase diagram of steady state networks for various underlying lattices and boundary conditions. In the main paper we presented results for one disordered lattice and several sizes. Here, we show results for a triangular lattice (Figs. 4, 9), the same disordered lattice as in the main paper but with $\gamma = 0.77$ (Fig. 5) and $\gamma = 0.59$ (Fig. 6), and a square lattice (Fig. 7). We choose boundary conditions where a single node is set to be a source and the remaining nodes sinks, as in the main paper. We position the single source at the center of the network to model animal tissues such as the retina and at the boundary to model a plant leaf (compare Fig. 4 in the main paper).

Our qualitative findings were robust, and did not depend on the choice of lattice or parameter $\gamma$.

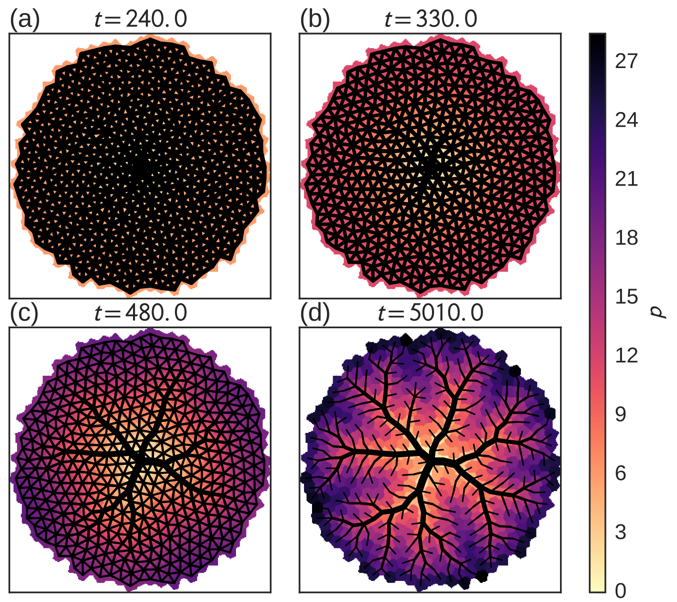


FIG. 3. Adaptation dynamics for a polynomial growth law with $n = 2$.

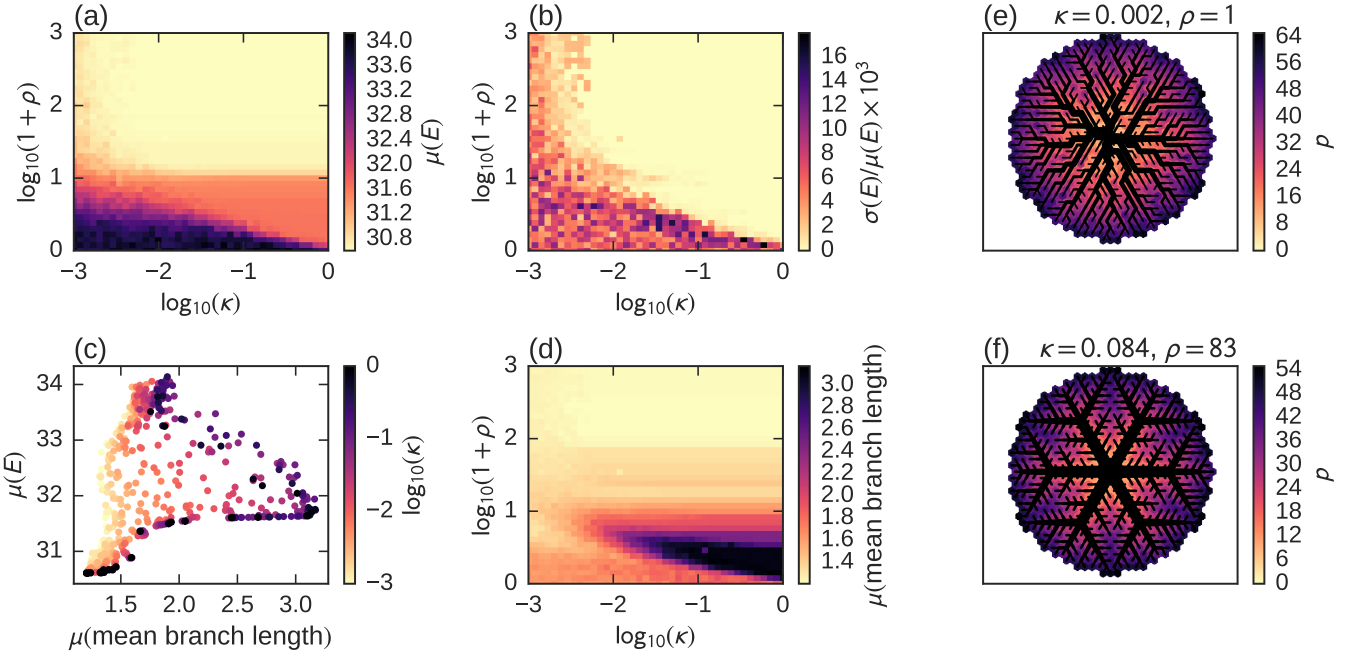


FIG. 4. (a) Energy landscape for a triangular lattice with approximately circular boundary and single source in the center, $\gamma = 2/3$, $N = 704$ nodes. (b) Relative standard deviation of the energy. (c) Mean branch length plotted against the energy. (d) Mean branch length landscape. (e,f) One disordered and one ordered example network.

### Generating disordered lattices

The disordered lattices were produced by initially randomly placing $N$ points (particles) on a 2D square surface. We then assumed a $1/r_{ij}^2$ repulsive potential between each pair of particles $\langle ij \rangle$. For each particle $k$, keeping all the other particles fixed, we found the new position $\vec{x}_k$ of the particle that minimizes the potential energy of the system, and updated the position $\vec{x}_k$. By sequentially updating the positions of all $N$ particles a sufficient amount of times we generated a list of node coordinates with a desired amount of disorder. The connectivity of the nodes and the

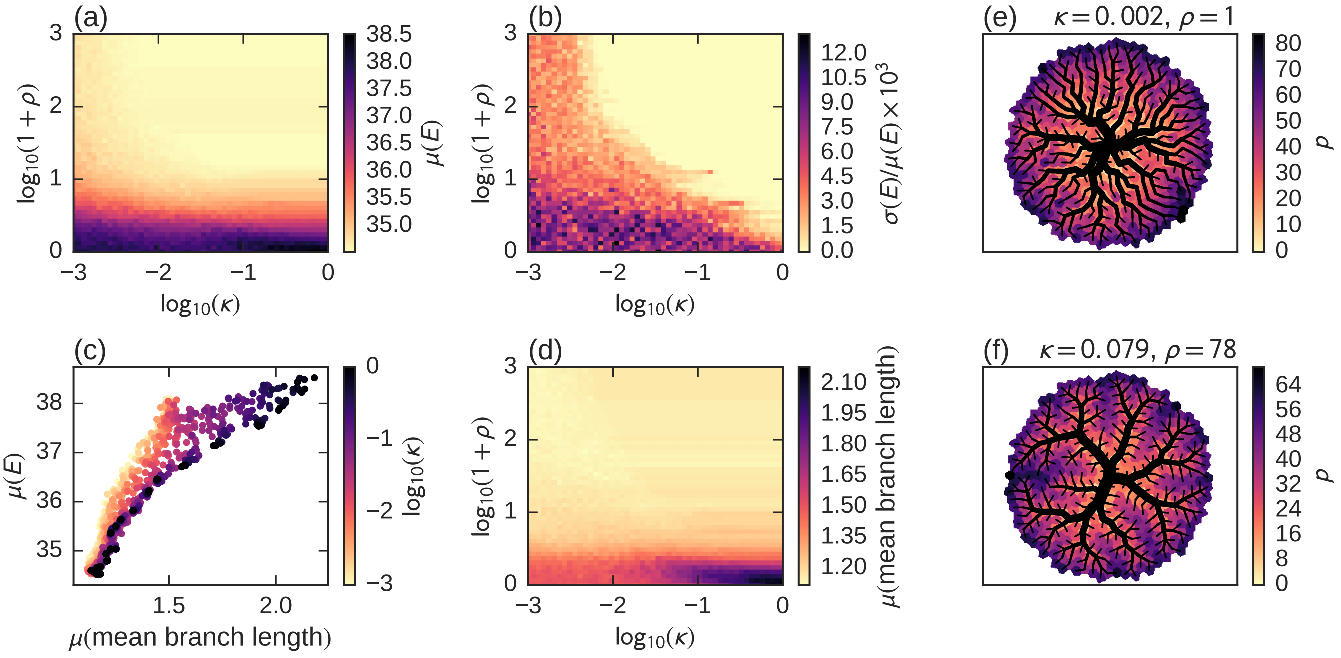


FIG. 5. (a) Energy landscape for a disordered lattice with approximately circular boundary and single source in the center, $\gamma = 0.77$, $N = 435$ nodes. (b) Relative standard deviation of the energy. (c) Mean branch length plotted against the energy. (d) Mean branch length landscape. (e,f) One disordered and one ordered example network.

tessellation units were determined from a Voronoi tessellation.

## X. FLUCTUATIONS AND LOOPS

In the manner of [4, 6, 7], it is possible to include fluctuations into the model by replacing $F_e^2 \to \langle F_e^2 \rangle$, where the angle brackets denote an average over configurations with different source vectors but the same set of conductivities. We show the resulting networks for the moving sink case where each configuration has a sink at one of the network nodes and a fixed source at the boundary in Fig. 11. As in the non-fluctuating case, growth leads to a higher degree of order in the network and to a network structure that closely resembles the highly optimized networks from [6, 7].


[1] Thomas Bittig, Ortrud Wartlick, Anna Kicheva, Marcos González-Gaitán, and Frank Jülicher. Dynamics of anisotropic tissue growth. *New Journal of Physics*, 10(6):063001, jun 2008.

[2] Shayn M Peirce and Thomas C Skalak. Microvascular remodeling: a complex continuum spanning angiogenesis to arteriogenesis. *Microcirculation (New York, N.Y. : 1994)*, 10(1):99–111, jan 2003.

[3] W J Hacking, E VanBavel, and J A E Spaan. Shear stress is not sufficient to control growth of vascular networks: a model study. *The American Journal of Physiology*, 270(1 Pt 2):H364–75, 1996.

[4] Dan Hu and David Cai. Adaptation and Optimization of Biological Transport Networks. *Physical Review Letters*, 111(13):138701, sep 2013.

[5] Anne-Gaëlle Rolland-Lagan and Przemyslaw Prusinkiewicz. Reviewing models of auxin canalization in the context of leaf vein pattern formation in Arabidopsis. *The Plant Journal*, 44(5):854–865, nov 2005.

[6] Eleni Katifori, Gergely J. Szöllősi, and Marcelo O. Magnasco. Damage and Fluctuations Induce Loops in Optimal Transport Networks. *Physical Review Letters*, 104(4):048704, jan 2010.

[7] Francis Corson. Fluctuations and Redundancy in Optimal Transport Networks. *Physical Review Letters*, 104(4):048703, jan 2010.

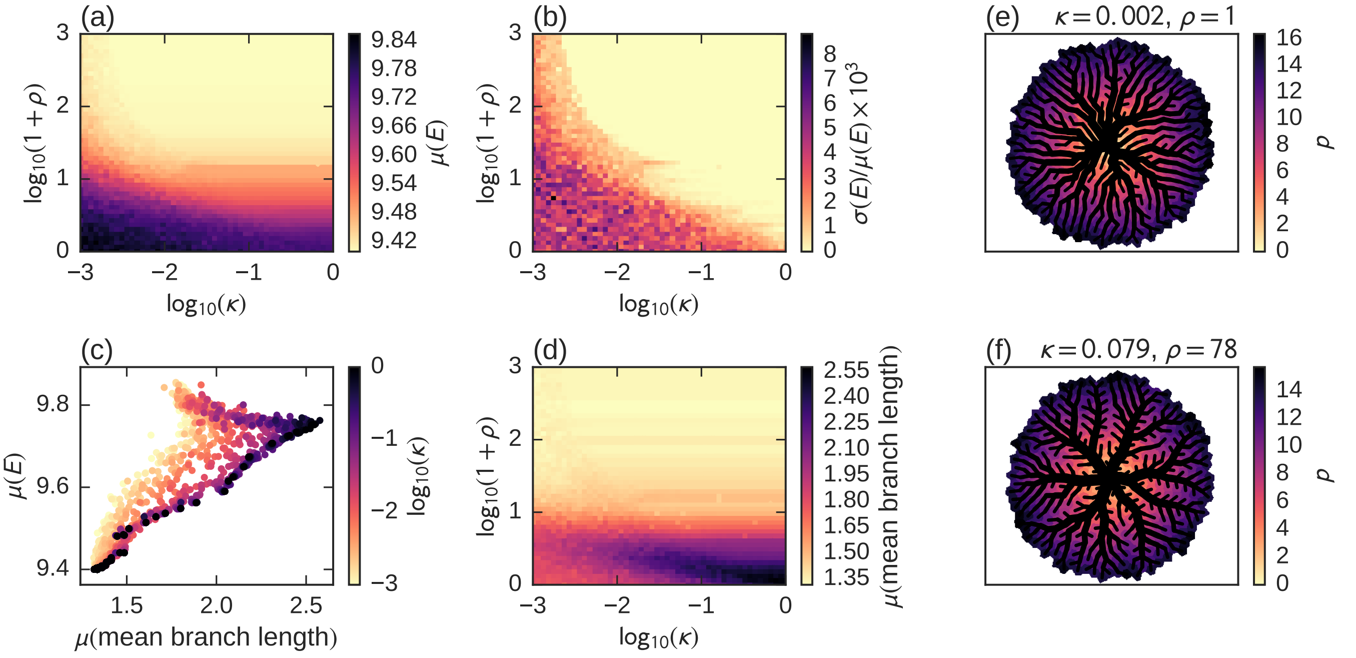


FIG. 6. (a) Energy landscape for a disordered lattice with approximately circular boundary and single source in the center, $\gamma = 0.59$, $N = 435$ nodes. (b) Relative standard deviation of the energy. (c) Mean branch length plotted against the energy. (d) Mean branch length landscape. (e,f) One disordered and one ordered example network.

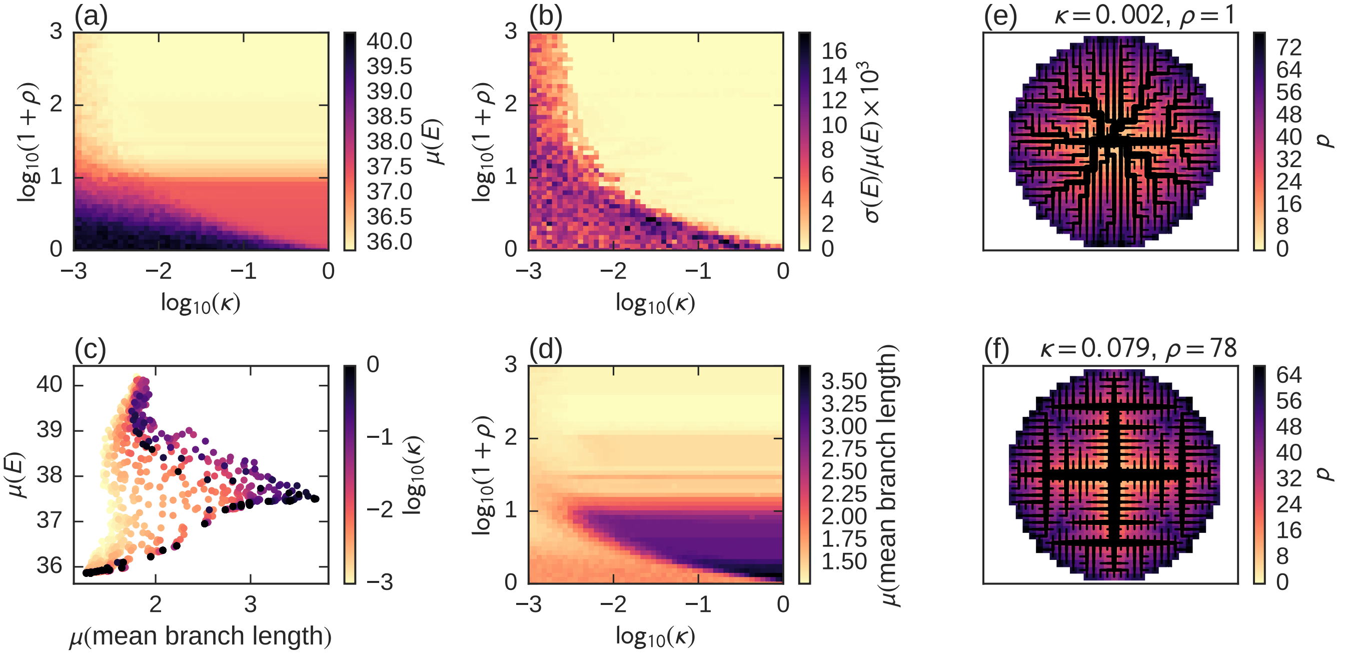


FIG. 7. (a) Energy landscape for a square lattice with approximately circular boundary and single source in the center, $\gamma = 2/3$, $N = 761$ nodes. (b) Relative standard deviation of the energy. (c) Mean branch length plotted against the energy. (d) Mean branch length landscape. (e,f) One disordered and one ordered example network.

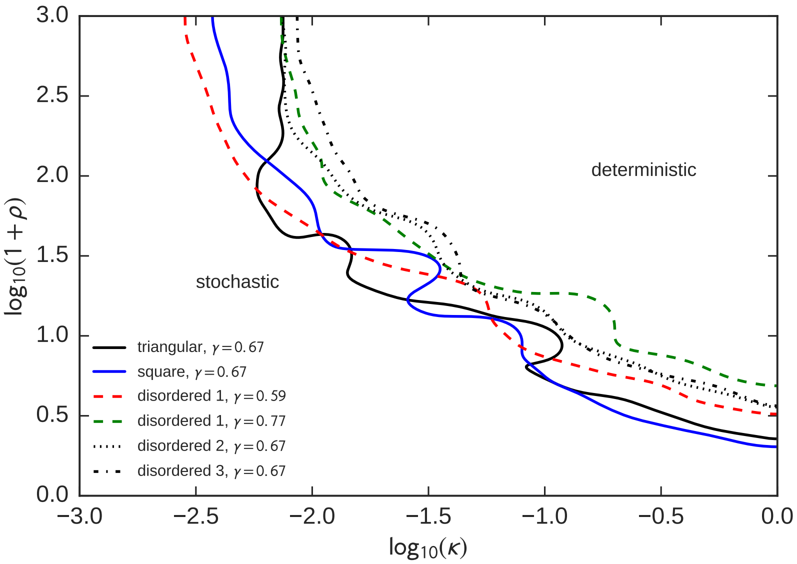


FIG. 8. The phase boundary between stochastic and deterministic states for networks with a single source at the center and approximately circular boundary. We plot the smoothed contour line where $\sigma(E)/\mu(E) = 10^{-4}$ for a triangular lattice (number of nodes $N = 704$), a square lattice ($N = 761$) and three different disordered lattices ($N = 435$, $N = 999$, $N = 1018$, respectively). For the first disordered lattice, we plot different values of $\gamma$. In general there is little variation in the position of the phase boundary.

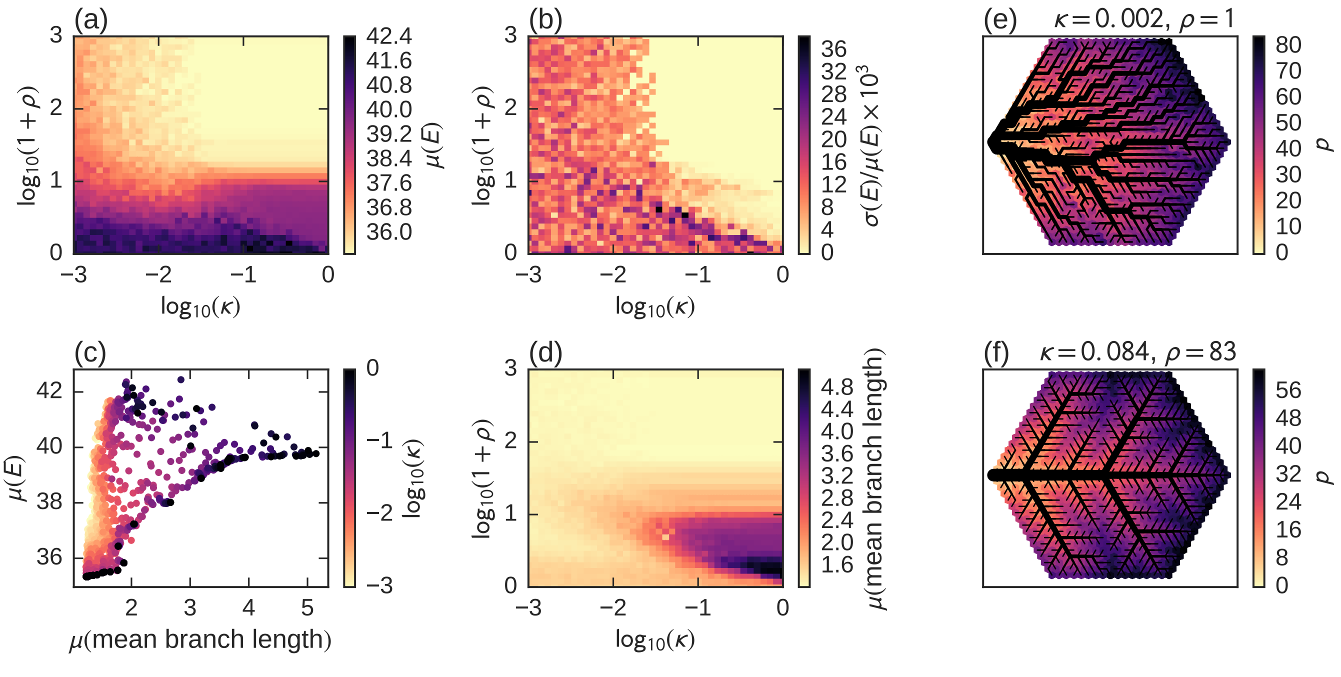


FIG. 9. (a) Energy landscape for a triangular lattice with hexagonal boundary and single source at one edge, $N = 817$ nodes. (b) Relative standard deviation of the energy. (c) Mean branch length plotted against the energy. (d) Mean branch length landscape. (e,f) One disordered and one ordered example network.

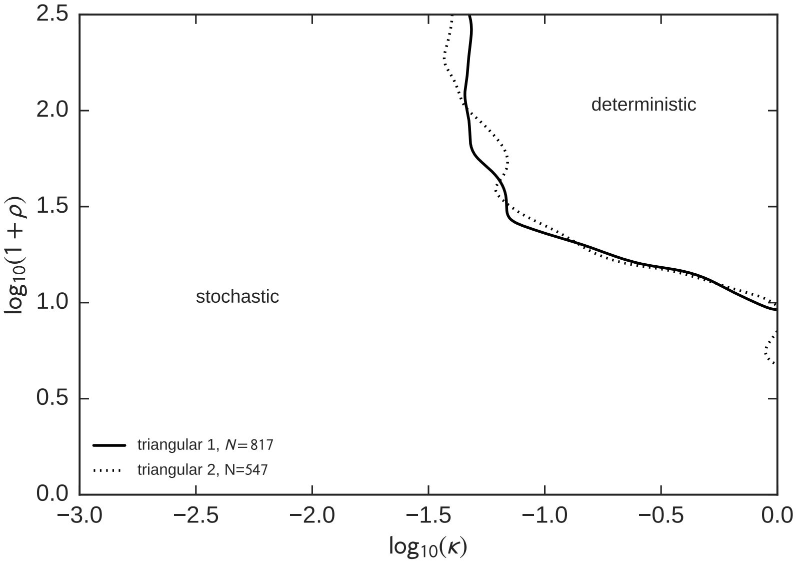


FIG. 10. The phase boundary between stochastic and deterministic states for networks with a single source at the edge and approximately hexagonal boundary. We plot the contour line where $\sigma(E)/\mu(E) = 10^{-4}$ for two triangular lattices of different size.

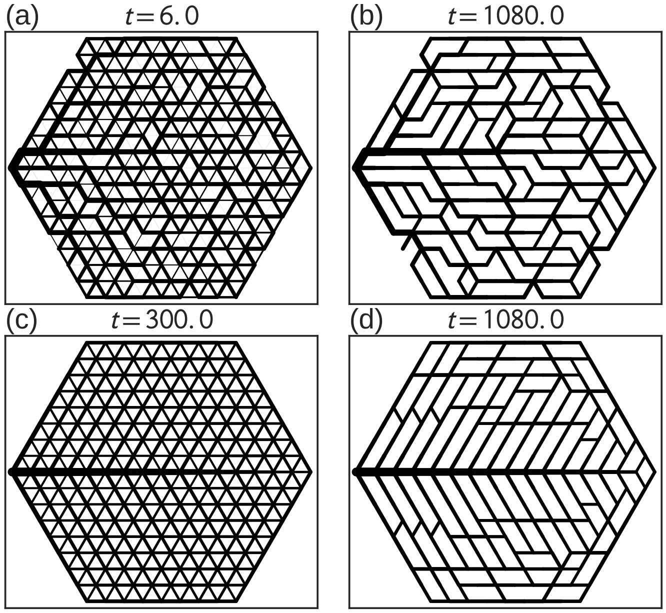


FIG. 11. Network dynamics with fluctuating flows and growth from random initial conditions. (a, b) Dynamics without growth, $\kappa = 0$. The resulting network is loopy but disordered, the dimensionless energy is $E' = 51.6$. (c, d) Dynamics with growth, $\kappa = 1, \rho = 50$. The resulting network remains loopy and shows a clear main vein but no secondaries, the dimensionless energy is $E' = 50.5$, a 2.0% improvement over the case without growth.
